# Supplementary material for: Few-shot Learning with Multilingual Language Models
Source: arXiv:2112.10668 source file (2022-11-10)
Supplement: Supplementary file 1 [file appendix_later.tex]

\hide{
\subsubsection{Comparison to XLM-R with Fine-tuning}
% \subsubsection{Comparison to Small Multilingual Language Models}
\label{sec:compare-to-small-lm}
% \xian{Should we change the section name to ``Comparison with XLM-R Finetuning"? I just feel our point is not to compare to a smaller model, but rather the existing finetuning approach.}
\begin{table*}[t!]
    \centering
    \scalebox{0.8}{
    \begin{tabular}{cc|ccccc|ccccc}
        \toprule
         & & \multicolumn{5}{c}{8-shot} & \multicolumn{5}{c}{16-shot} \\
         model & method & zh & tr & ur & sw & Avg & zh & tr & ur & sw & Avg. \\
         \midrule
         \multirow{3}{*}{\makecell{XLM-R base 270M\\~\cite{DBLP:journals/corr/abs-2109-03630}}} & FT & 33.3 & 32.8 & 32.8 & 32.7 & 32.9 & 33.6 & 33.8 & 33.5 & 33 & 33.5    \\
         & DP & 37.5 & 38.0 & 39.3 & 33.8 & 37.2 & 42.2 & 39.4 & 40.6 & 34.5 & 39.2 \\
         & SP & 34.4 & 35.4 & 34.6 & 33.5 & 34.5 & 35.6 & 40.2 & 35.5 & 34.0 & 36.3 \\
         \midrule
         \makecell{\Ours 564M}& IC$^\dagger$ & 35.1 & 35.5 & 37.2 & 38.7 & 36.6 & 35.4 & 36.2 & 38.4 & 38.8 & 37.2 \\
         \makecell{\Ours 7.5B} & IC$^\dagger$ & \highest{51.7} & \highest{48.3} & \highest{46.5} & \highest{47.3} & \highest{48.5} & \highest{52.0} & \highest{46.4} & \highest{46.7} & \highest{46.9} & \highest{48} \\
         \bottomrule
    \end{tabular}
    }
    \caption{Comparison to XLM-R with fine-tuning~\cite{DBLP:journals/corr/abs-2109-03630} on XNLI (\lang{zh}, \lang{tr}, \lang{ur} and \lang{sw}). In this table, $k$-shot is defined as $k$ examples per class. We report the mean of our model over 5 different runs corresponding to different training sets. % sampled from the the XNLI development split. 
    \texttt{FT}: fine-tuning; \texttt{DP}: discrete prompting; \texttt{SP}: soft prompting; \texttt{IC}: in-context learning. $^\dagger$ We pick \lang{en} prompts for all languages based on the performance on the original XNLI development set, while~\citet{DBLP:journals/corr/abs-2109-03630} uses a few-shot development set.}
    \label{tab:comparison-to-xlmr-base-in-language-xnli}
\end{table*}

\paragraph{XLM-R with fine-tuning.} Previous work has shown that small language models % which can be trained with much less computation 
are also few-shot learners when combined with % cloze-style task reformulation and 
gradient-based optimization~\cite{DBLP:journals/corr/abs-2009-07118,DBLP:journals/corr/abs-2109-03630}. We compare the few-shot learning performance of \Ours to the fine-tuned XLM-R (270M) model~\cite{DBLP:journals/corr/abs-2109-03630} on the XNLI task (\S\ref{sec:compare-to-small-lm}).

We also compare % the few-shot learning performance of \Ours 
to the \xlmrbase model~\cite{conneau-etal-2020-unsupervised} combined with full-finetuning (FT), discrete prompting (DP) and soft prompting (SP) as proposed by~\citet{DBLP:journals/corr/abs-2109-03630}. % , using the same experiment setting as theirs: 
We directly compare to the results reported by~\citet{DBLP:journals/corr/abs-2109-03630}, by evaluating on a subset of languages (\lang{zh}, \lang{tr}, \lang{ur}, \lang{sw}) of the XNLI dataset and sampling $k$ examples \emph{per class}for few-shot training.\footnote{We compared the $k$-shot \emph{per class} setup % and the majority label bias~\cite{DBLP:conf/icml/ZhaoWFK021} problem 
to the $k$-shot \emph{in total} setup used in the rest of the paper in Appendix~\ref{sec:few-shot-training-set-distribution}.}  
There are some important differences in our design choices. Our XNLI prompts, as shown in Table~\ref{tab:multilingual_prompts}, are different from those used by~\citet{DBLP:journals/corr/abs-2109-03630}, which were in turn taken from~\citet{DBLP:journals/corr/abs-2103-10385}. Besides, we use the English prompts for all languages based on the performance on the original XNLI development set (\S\ref{sec:multilingual_prompt_construction}), while~\citet{DBLP:journals/corr/abs-2109-03630} uses Google-translated prompts for non-English languages.

As shown in Table~\ref{tab:comparison-to-xlmr-base-in-language-xnli}, with about twice the parameters of \xlmrbase, \model{\Oursns}{564M} with in-context learning outperforms \xlmrbase combined with FT and SP, but underperforms \xlmrbase combined with DP (averaged across the languages). Scaling up the parameter size offers tremendous performance boost. \model{\Oursns}{7.5B} outperforms \xlmrbase combined with DP by 30.4\% in the 8-shot setting and 22.4\% in the 16-shot setting, despite using no gradient updates. % However, the comparison to our models at both 564M and 7.5B scales indicates that the main factor contributing to the superior performance of our largest model is parameter size instead of the prompt difference.}. % Moreover, our models can also be combined with FT, DP and SP. We leave the investigation of efficient fine-tuning of large-scale multilingual language models to future work.}. 
While our largest model outperforms~\citet{DBLP:journals/corr/abs-2109-03630} by a large margin, its performance slightly drops going from 8-shot to 16-shot, echoing the trend shown in Figure~\ref{fig:multi_few_shot_by_resource_level} that larger $k$'s do not always lead to significantly better performance. 
% that larger values of $k$ do not always yield better performance.
The performance of all fine-tuning based approaches (FT, DP and SP) significantly improves as the number of training examples increases as expected. Our models can be combined with FT, DP and SP. We leave the investigation of efficient fine-tuning of large-scale multilingual language models to future work.
}
